# Supplementary material for: Mosaic: Composite Projection Pruning for Resource-efficient LLMs
Source: arXiv:2504.06323 source file (2025-08-12)
Supplement: Supplementary file 1 [file supplementary.tex]

\noindent {\Large \textbf{Supplementary Materials}}
\section*{Hardware Platforms Detailed}
